# Supplementary material for: Whispering Pixels: Exploiting Uninitialized Register Accesses in Modern GPUs
Source: arXiv:2401.08881 source file (2024-01-16)
Supplement: Supplementary file 1 [file appendix.tex]

\section{Appendix}
\label{sec:appendix}
